# Supplementary material for: Incorporating Terminology Constraints in Automatic Post-Editing
Source: arXiv:2010.09608 source file (2020-10-19)
Supplement: Supplementary file 1 [file appendix.tex]

\clearpage
\newpage
\appendix

\section{Result on regular APE using constrained variants}
We evaluate our constrained APE systems on the regular PBMT and NMT tasks without supplying any terminologies. For Append and Replace, a stream of source tokens 1 are supplied. The only change to MS LevT is the initialization during inference. Instead of the list of terminologies, the model starts with a blank sentence. See \autoref{result_pbmt_regular} and \autoref{result_nmt_regular} for the results on PBMT and NMT tasks respectively. For PBMT, the constrained models perform slightly better than the unconstrained version despite not having the terminologies as input. On NMT, only the replace method gains some TER and BLEU. The LevT model is improved, but still unperformed than the do-nothing case.

\begin{table}[t]
\begin{center}
\begin{tabular}{l c c c c }
\toprule
 & Term\% & TER & BLEU   \\
\midrule
Do-nothing & 88.48 & 24.25 & 62.99 \\
MS\_UEdin\ & 88.70 & \textbf{18.01} & \textbf{72.52} \\
\midrule
MST & 90.11 & 19.34 & 70.44 \\
MST Append & \textbf{91.50} & \textbf{18.77} & \textbf{70.85} \\
MST Replace & 90.90 & 19.25 & 70.53 \\
\midrule
LevT  & 90.76 & 24.21 & 63.47 \\
LevT App & 89.17 & 24.10 & 64.72 \\
LevT Rep  & 89.17 & 23.76 & 65.27 \\
MS LevT & 89.83 & 20.59 & 68.59 \\
\bottomrule
\end{tabular}
\end{center}
\caption{\label{result_pbmt_regular} Results for PBMT 2018. The constrained systems do not receive any terms as input.  }
\end{table}
\begin{table}[t]
\begin{center}
\begin{tabular}{l c c c c }
\toprule
 & Term\% & TER & BLEU  &  \\
\midrule
Do-nothing & 90.22 & 16.84 & 74.73 \\
Unbabel\_BERT & 89.98  & \textbf{16.06} & \textbf{75.96}  \\
\midrule
MST & 90.66 & 16.46 & 75.61 \\
MST Append  & 90.89 & 16.57 & 75.21 \\
MST Replace & 89.98 & 16.42 & 75.65 \\
\midrule
MS LevT & 89.98 & 17.17 & 74.46 \\
\bottomrule
\end{tabular}
\end{center}
\caption{\label{result_nmt_regular} Results for NMT 2019. The constrained systems do not receive any terms as input. }
\end{table}

\section{Levenshtein Transformer}

\subsection{PBMT 2017}
We present our results on PBMT 2017 task, which the Levenshtein Transformer experimented with APE task. Our MST models all outperform the SOTA. The regular LevT models with and without constraints is only able to outperform the do-nothing case by a small margin.
\begin{table}[h]
\begin{center}
\begin{tabular}{l c c c c }
\hline
 & term\% & TER & BLEU   \\
\hline
Do-nothing & 88.83 & 24.48 & 62.49 \\
\hline
MST  & 90.83 & 18.83 & 71.07 \\
MST Append  & 95.83 & 18.60 & 71.02 \\
MST Replace & 95.50 & 19.13 & 70.61 \\
\hline
LevT  & 89.50 & 24.45 & 65.31\\
LevT App. & 91.00 & 24.04 & 64.80 \\
LevT Rep.  & 91.00 & 23.76 & 65.31 \\
MS LevT & 98.17 & 20.53 & 68.66\\

\end{tabular}
\end{center}
\caption{\label{result_pbmt_2017} Results for PBMT 2017.  }
\end{table}

\subsection{Distillation}
We experimented with the use of a distillation dataset to improve the performance of Multi-source Levenshtein Transformer. Due to the dual training aspect of APE, we have the pretrained and finetuned models as candidates for the autoregressive teacher. We tested with different combinations of autoregressive teachers for pretraining and finetuning. In addition to the two teachers, we also experiment with the output generated by the append model.

\begin{table}[h]
\begin{center}
\begin{tabular}{c c c c c}
\hline
Pretrain & Finetune & term\% & TER & BLEU \\
\hline
 - & - & 98.04 & 17.71 & 73.64 \\
 - & ft. &  97.72 & 17.91 & 73.26 \\
 - & app. &  97.72 & 17.87 & 73.31 \\
 pre. & - & 99.09 & 17.17 & 74.40 \\
 pre. & ft. &  \textbf{99.54}  & 17.09 & 74.29\\
 pre. & app. &  \textbf{99.54} & 17.07 & 74.32 \\
 ft. & - &  96.81 & 17.06 & 74.48 \\
 ft. & ft. & 96.13 & 17.04 & 74.48 \\
 ft. & app. &  96.13 & \textbf{17.02} & \textbf{74.52} \\
 app. & - &  98.41 & 17.11 & 74.40 \\
 app. & app. &  98.86 & 17.24 & 74.04 \\

\end{tabular}
\end{center}
\caption{\label{result_distillation} Experiments with distillation. We show the distillation teacher for pretraining and finetuning. The teachers include pretrained baseline model (pre.), finetuned baseline model (ft.), and the append method (app.). }
\end{table}

\autoref{result_distillation} shows the results of APE NMT for the different combinations. First, distillation is crucial at pretraining, as finetuning with distillation on the original pretrained model hurts the performance. For terminology constraints, the best performing model is using the respective teacher model for each step. This combination that mirrors the actual learning also helps to lower the TER by 0.70. The best gain is seen is when the finetuned distillation dataset is also used for pretraining. However, the model is still not able to perform better than the do-nothing case. We leave this for further investigation for future works.
